# Supplementary material for: Spatial Privacy Pricing: The Interplay between Privacy, Utility and Price in Geo-Marketplaces
Source: arXiv:2008.11817 source file (2020-09-04)
Supplement: Supplementary file 1 [file 07-supplementary.tex]

\begin{appendix}
\section{Appendix}
\knremovepomdp{I removed the section about POMDP and modelling our problem as a POMDP.}

\subsection{Additional Experiment Results}
\label{subsec:sup:more_results}
This section shows the recall comparison between algorithms for different parameters. The general trend is that SIP and SIP-T consistently achieve good recall. 
The result for the gross margin per user $\uprofit$ is shown in Table~\ref{tbl:exp_vary_profit_per_user_recall}, for the size $\regionsize$ of the target region is shown in Table~\ref{tbl:exp_vary_grid_cell_len_recall}, for the scale $\privscale$ of the privacy distributions is shown in Table~\ref{tbl:exp_vary_privacy_valuation_scale_recall}, for the starting price $\price_0$ is shown in Table~\ref{tbl:exp_vary_start_price_recall}, for the price increment factor $\priceincreasefactor$ is shown in Table~\ref{tbl:exp_vary_price_increment_factor_recall}.
\kn{I will write more about these tables later}

\subsection{Illustration of Check-ins of Users}
\label{subsec:sup:checkins}
Figure~\ref{fig:checkins_LA_1_per_user} shows the check-ins in Los Angeles area within the bounding box, converted to local Euclidean coordinates. There are total 5827 users and each user has one check in selected randomly from their check-ins. The method is explained as follows:

A subtended degree in latitude and longitude represents different arc lengths on the earth, so we converted the latitude/longitude coordinates in each check-in to  local Euclidean coordinates $(x, y)$ in meters. Using a reference origin point of $(lat_0,long_0)$ and an assumption of a spherical earth, the local Euclidean coordinates $(x, y)$ of the point $(lat,long)$ are
\begin{align}
    x &= R\cos(lat_0)(long - long_0) \\
    y &= R(lat - lat_0)
\end{align}
    
\noindent
where $R$ is the radius of the earth in meters. The reference $(lat_0,long_0)$ was chosen as the mid-point of the latitude/longitude bounding box. The bounding box in local Euclidean coordinates $(x, y)$ is from the southwest corner at (-25,000, -35,000) to the the northeast corner at (25,000, 35,000) in meters. 

\begin{figure}[htbp!]
\centering
\includegraphics[width=.5\linewidth]{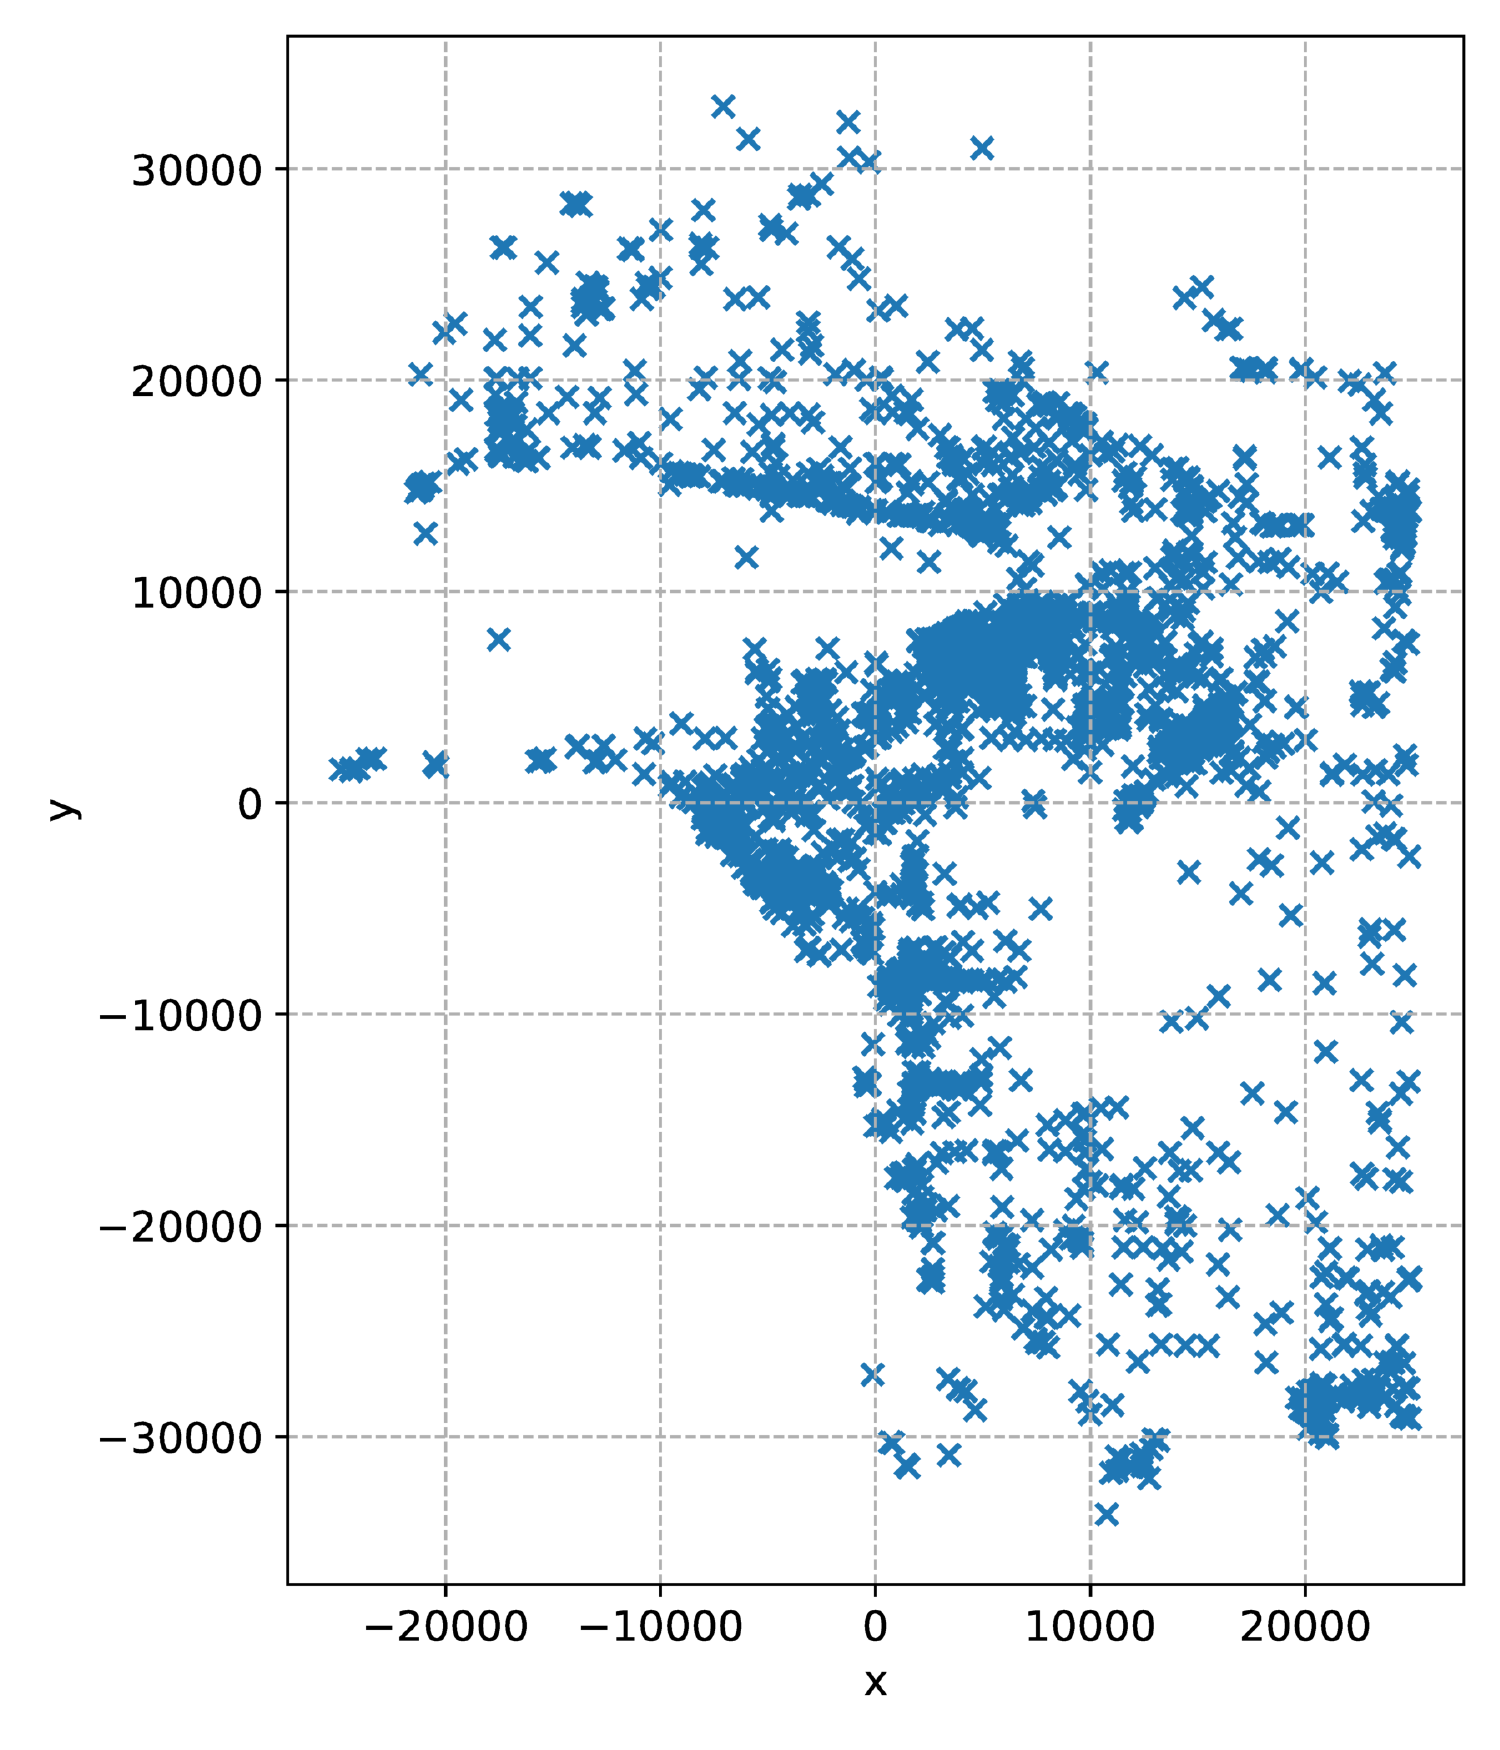}
\caption{Check-ins of Gowalla users in Los Angeles converted to local Euclidean coordinates, 1 check-in per user.} 
\label{fig:checkins_LA_1_per_user}
\end{figure}

\end{appendix}
